# Supplementary material for: Energy-ordered resource stratification as an agnostic signature of life
Source: arXiv:2403.18614 source file (2024-12-23)

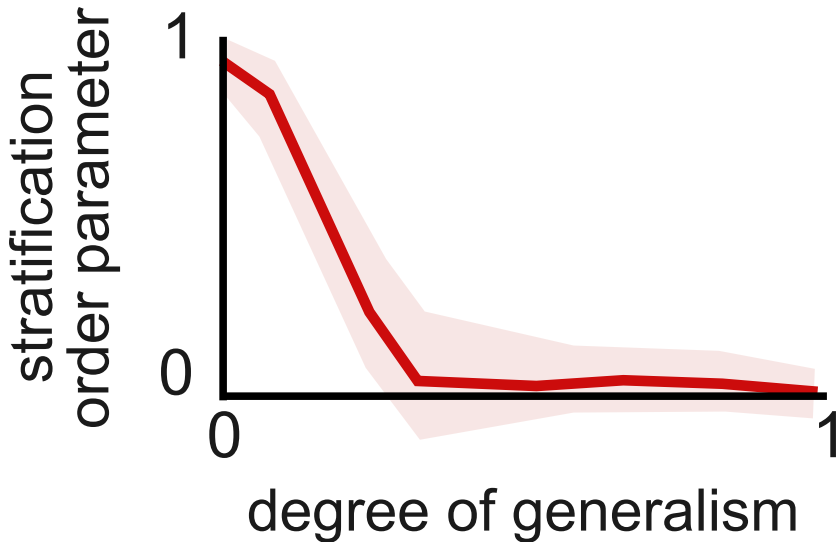

Resource Concentrations

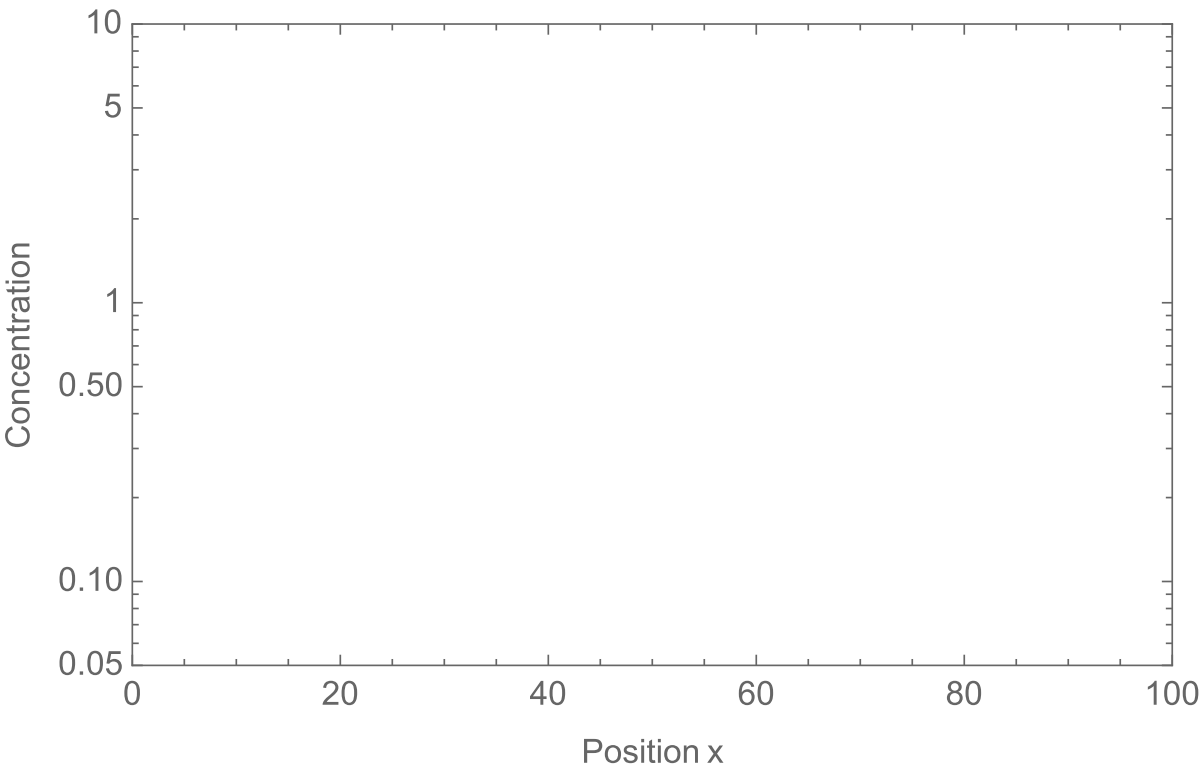

Species Abundances

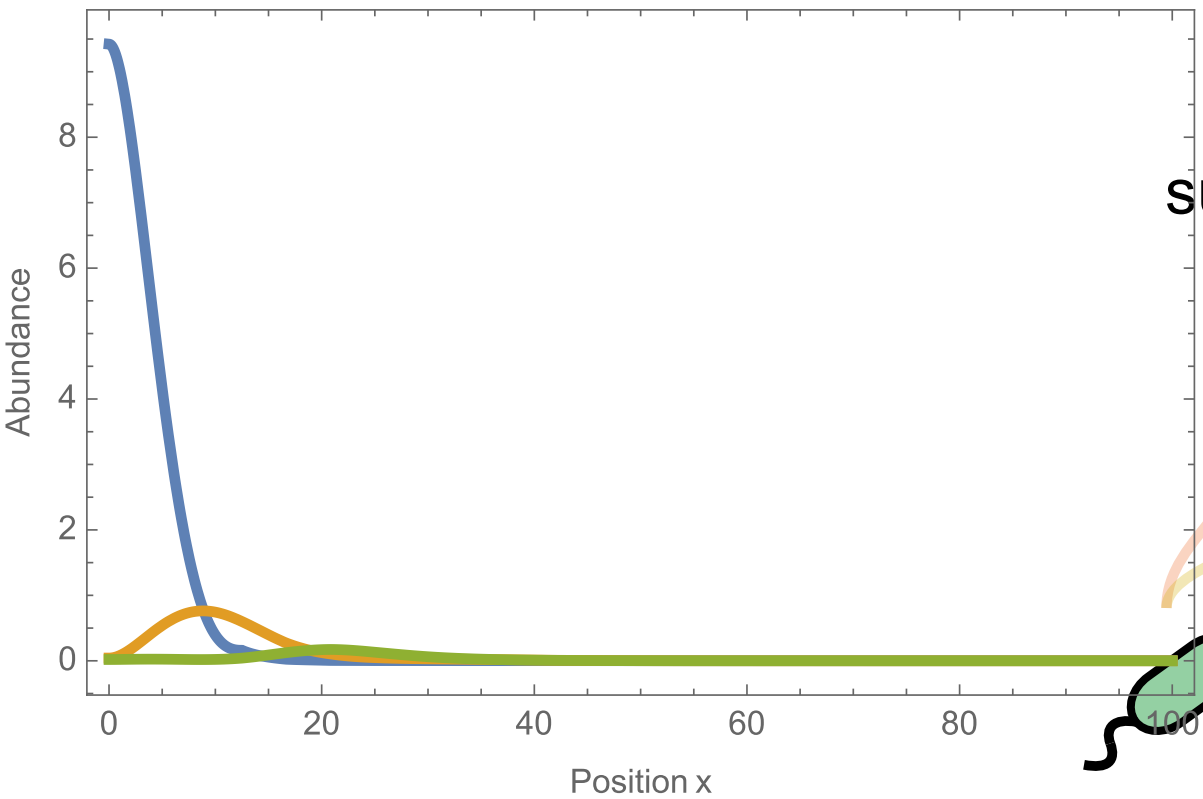

Supplement: Supplementary file 1 [file si_001_generalists.pdf]
