# Supplementary material for: Energy-ordered resource stratification as an agnostic signature of life
Source: arXiv:2403.18614 source file (2024-12-23)

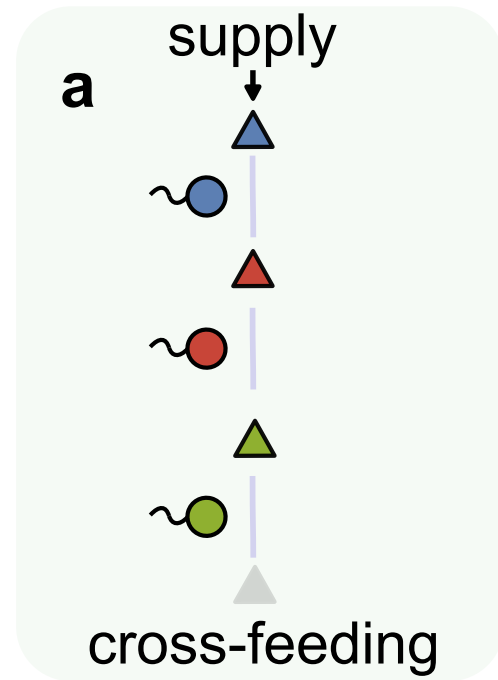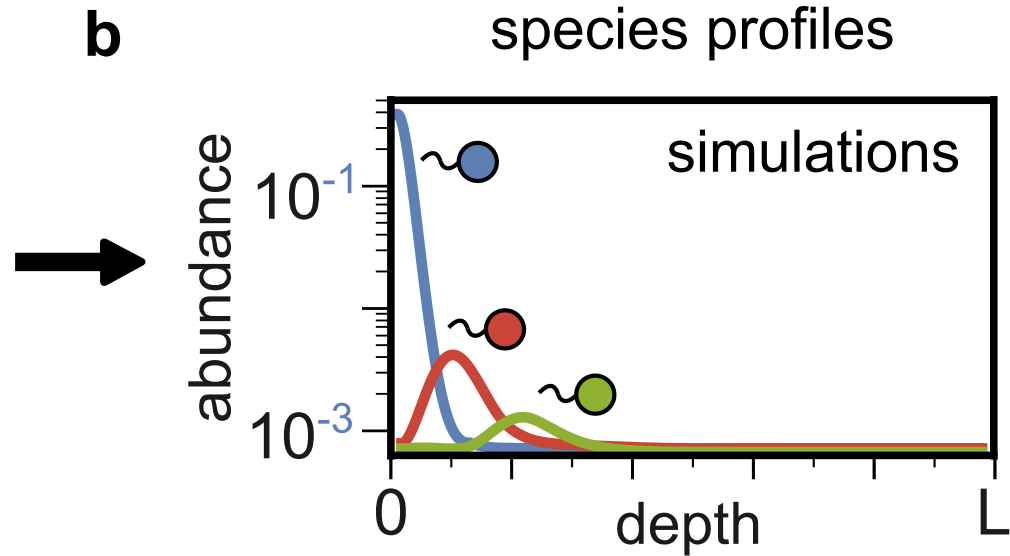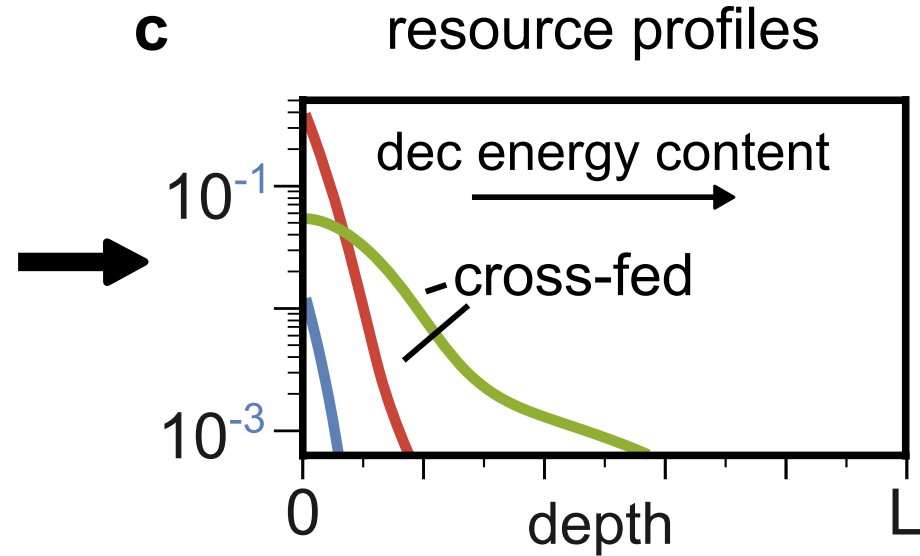

# Resource Concentrations

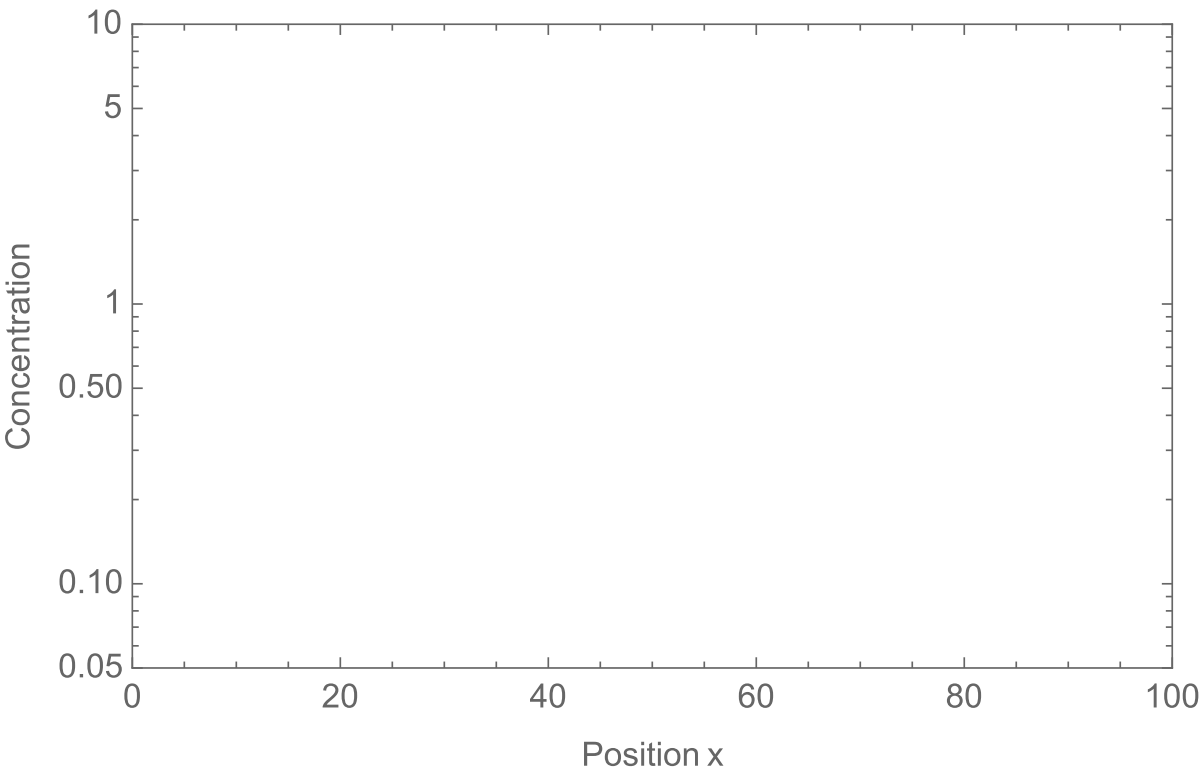

# Species Abundances

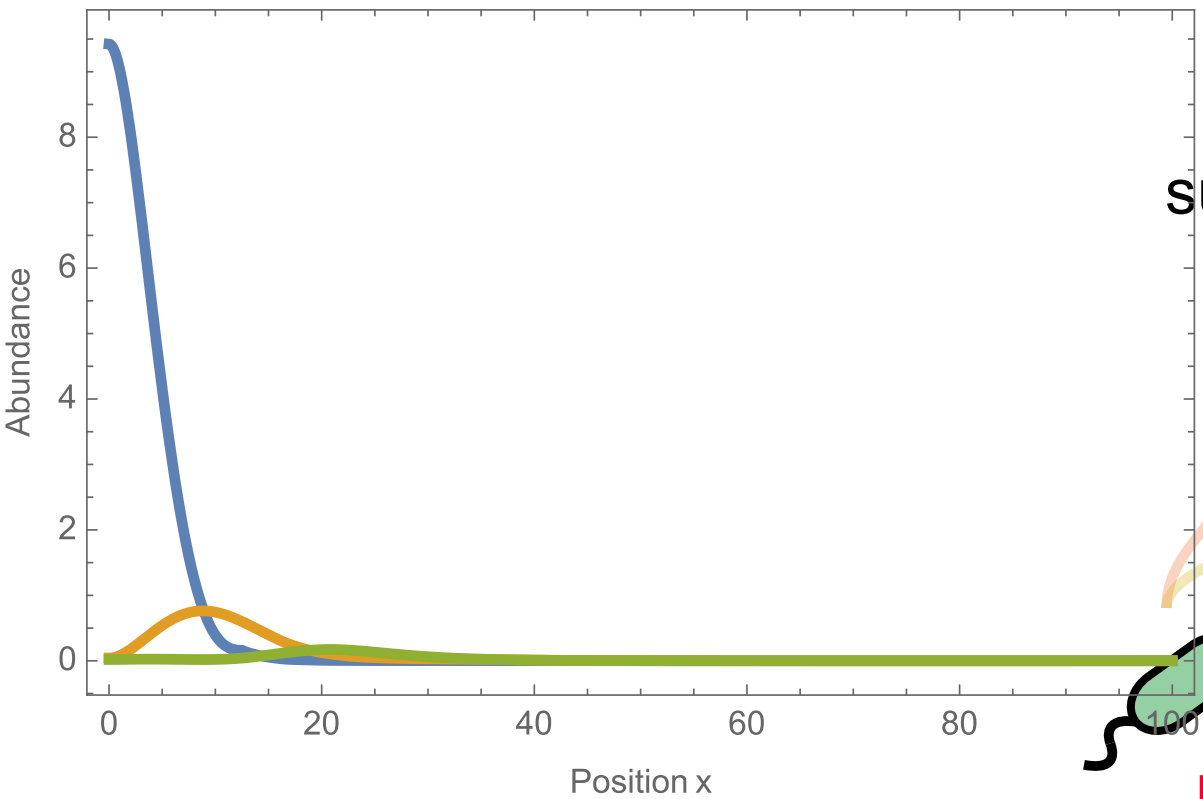

Supplement: Supplementary file 2 [file si_002_cross_feeding.pdf]
